# Supplementary material for: No alignment of cattle along geomagnetic field lines found
Source: arXiv:1101.5263 ancillary file (2011-02-01)
Supplement: Supplementary file 1 [file Online_Resource_1.pdf]

# Supporting material for the manuscript "Hert J, Jelinek L, Pekarek L, Pavlicek A (2010) No alignment of cattle along geomagnetic field lines found. Journal of Comparative Physiology - A".

## 1) Herd-axes angles of 110 herds corresponding to Fig. 1a (angles are measured in degrees from east to west in counter-clockwise sense)

89, 113, 66, 68, 118, 128, 39, 179, 108, 46, 167, 64, 74, 143, 36, 148, 69, 133, 126, 29, 146, 155, 118, 49, 83, 159, 144, 94, 163, 60, 19, 141, 149, 71, 68, 50, 84, 122, 75, 2, 163, 10, 2, 48, 13, 122, 58, 98, 175, 149, 34, 155, 140, 153, 168, 175, 50, 112, 78, 37, 55, 179, 91, 146, 98, 166, 153, 16, 172, 77, 158, 51, 123, 136, 101, 158, 34, 22, 47, 18, 4, 126, 98, 13, 155, 31, 60, 41, 132, 6, 3, 127, 46, 92, 65, 139, 133, 60, 94, 155, 87, 111, 86, 139, 50, 155, 102, 34, 55, 9

## 2) Herd-axes angles of 110 herds corresponding to Fig. 1b (angles are measured in degrees from east to west in counter-clockwise sense)

78, 167, 101, 111, 51, 71, 154, 76, 131, 178, 156, 65, 33, 53, 59, 54, 125, 55, 138, 179, 36, 72, 143, 76, 127, 82, 57, 79, 72, 69, 80, 60, 50, 39, 122, 36, 84, 18, 92, 75, 88, 142, 91, 123, 35, 66, 29, 56, 116, 174, 144, 29, 159, 61, 166, 10, 152, 136, 32, 94, 164, 163, 73, 49, 169, 88, 161, 37, 124, 42, 15, 44, 93, 100, 116, 131, 52, 63, 97, 26, 26, 154, 163, 67, 18, 91, 118, 26, 105, 16, 146, 79, 95, 48, 124, 125, 134, 137, 102, 65, 1, 161, 108, 34, 139, 119, 99, 98, 106, 114

## 3) Body-axes angles of 1636 cows corresponding to Fig. 2a (angles are measured in degrees from east to west in counter-clockwise sense)

60, 105, 92, 92, 63, 88, 51, 93, 92, 116, 116, 67, 125, 53, 82, 108, 63, 112, 61, 100, 98, 94, 91, 121, 74, 90, 136, 131, 119, 96, 179, 116, 180, 122, 142, 77, 124, 100, 67, 53, 93, 50, 33, 100, 179, 123, 176, 118, 114, 64, 151, 92, 7, 31, 162, 64, 54, 78, 62, 55, 58, 82, 82, 63, 71, 91, 144, 57, 48, 50, 164, 67, 89, 87, 67, 55, 83, 161, 119, 114, 121, 153, 156, 87, 46, 73, 124, 143, 166, 6, 128, 114, 94, 91, 132, 46, 52, 92, 140, 89, 91, 133, 143, 82, 140, 127, 114, 105, 106, 126, 9, 117, 101, 128, 112, 101, 14, 17, 120, 149, 135, 144, 165, 61, 29, 49, 50, 158, 81, 67, 53, 24, 25, 161, 60, 35, 31, 143, 100, 36, 33, 52, 50, 168, 2, 12, 29, 59, 163, 130, 29, 64, 122, 148, 112, 157, 105, 68, 167, 159, 14, 140, 3, 171, 144, 142, 90, 36, 160, 147, 109, 105, 141, 142, 96, 167, 90, 94, 105, 41, 103, 22, 31, 45, 43, 176, 81, 83, 89, 77, 29, 155, 96, 87, 75, 79, 92, 5, 100, 69, 39, 75, 152, 71, 161, 44, 27, 15, 68, 106, 140, 138, 131, 89, 168, 178, 58, 56, 94, 89, 3, 40, 152, 135, 7, 170, 168, 153, 65, 177, 158, 27, 154, 95, 88, 95, 106, 148, 29, 57, 5, 159, 23, 124, 65, 87, 31, 53, 104, 48, 13, 137, 102, 45, 56, 11, 126, 26, 158, 97, 137, 102, 71, 127, 99, 76, 157, 140, 85, 98, 147, 84, 80, 38, 100, 133, 101, 99, 125, 132, 98, 96, 93, 95, 170, 151, 1, 73, 43, 103, 170, 137, 119, 37, 91, 146, 31, 120, 54, 170, 175, 133, 81, 55, 22, 159, 94, 86, 101, 1, 45, 82, 92, 73, 65, 87, 102, 32, 28, 97, 36, 47, 77, 136, 147, 180, 101, 152, 145, 150, 162, 89, 126, 61, 48, 142, 57, 42, 74, 105, 125, 179, 81, 81, 37, 102, 105, 127, 134, 142, 109, 112, 143, 83, 30, 93, 169, 157, 15, 98, 151, 146, 0, 37, 111, 168, 63, 134, 10, 131, 66, 15, 71, 14, 140, 23, 93, 10, 164, 50, 6, 52, 158, 59, 44, 111, 136, 128, 140, 32, 129, 147, 0, 53, 178, 31, 156, 167, 7, 86, 102, 33, 152, 62, 76, 149, 120, 161, 39, 23, 43, 5, 2, 51, 149, 82, 65, 127, 159, 135, 62, 153, 83, 72, 177, 139, 160, 171, 106, 178, 126, 138, 162, 160, 153, 144, 36, 104, 18, 172, 155, 79, 56, 125, 50, 38, 116, 37, 136, 126, 160, 131, 11, 32, 150, 171, 136, 138, 146, 94, 168, 138, 158, 173, 63, 122, 152, 119, 141, 168, 174, 16, 7, 4, 171, 169, 164, 0, 32, 3, 8, 124, 85, 100, 136, 170, 112, 161, 97, 139, 29, 13, 133, 167, 15, 176, 173, 25, 105, 169, 76, 129, 77, 138, 57, 4, 175, 119, 58, 70, 69, 74, 69, 23, 107, 144, 129, 5, 155, 20, 168, 179, 148, 147, 176, 139, 122, 132, 97, 83, 127, 19, 123, 43, 2, 39, 110, 80, 117, 55, 30, 143, 142, 105, 155, 99, 89, 100, 80, 64, 58, 39, 55, 94, 105, 13, 65, 79, 64, 62, 132, 125, 39, 121, 132, 130, 24, 9, 150, 146, 180, 131, 135, 130, 149, 132, 138, 114, 23, 95, 176, 37, 51, 123, 99, 138, 108, 67, 105, 119, 67, 59, 43, 74, 126, 67, 41, 115, 44, 124, 102, 41, 60, 64, 50, 40, 55, 179, 57, 153, 118, 77, 66, 78, 50, 118, 105, 55, 128, 179, 55, 53, 109, 124, 19, 96, 4, 13, 11, 172, 22, 100, 110, 91, 71, 89, 50, 102, 105, 99, 43, 81, 71, 60, 177, 120, 163, 93, 6, 153, 9, 44, 1, 176, 160, 136, 167, 7, 18, 19, 13, 104, 3, 86, 2, 129, 170, 12, 16, 146, 92, 31, 5, 56, 29, 118, 118, 4, 161, 93, 18, 16, 5, 108, 158, 33, 63, 71, 116, 21, 100, 30, 31, 22, 53, 157, 117, 96, 100, 119, 45, 44, 83, 78, 47, 95, 69, 44, 100, 40, 87, 133, 120, 1, 38, 116, 103, 121, 135, 99, 39, 139, 138, 42, 33, 37, 173, 165, 19, 159, 71, 79, 47, 33, 115, 150, 114, 87, 139, 145, 4, 143, 69, 7, 35, 39, 65, 134, 68, 115, 100, 49, 154, 36, 30, 50, 32, 143, 123, 167, 169, 2, 2, 57, 43, 57, 100, 38, 91, 41, 144, 116, 166, 132, 167, 171, 103, 171, 163, 174, 128, 151, 4, 108, 133, 130, 123, 122, 108, 106, 150, 139, 144, 170, 105, 177, 135, 78, 33, 145, 160, 146, 178, 142, 179, 26, 166, 117, 30, 178, 146, 33, 153, 155, 144, 129, 169, 120, 136, 127, 94, 165, 129, 16, 143, 3, 175, 69, 129, 160, 147, 159, 151, 24, 159, 165, 10, 155, 8, 138, 40, 48, 113, 16, 42, 47, 170, 55, 45, 69, 118, 39, 61, 0, 169, 97, 109, 128, 115, 87, 70, 154, 31, 48, 89, 66, 178, 157, 6, 99, 117, 162, 62, 3, 37, 59, 135, 148, 136, 59, 56, 73, 114, 7, 88, 125, 54, 41, 136, 62, 57, 30, 24, 178, 39, 40, 56, 28, 6, 89, 39, 59, 27, 11, 33, 79, 152, 163, 160, 59, 1, 30, 145, 39, 66, 121, 87, 84, 163, 89, 63, 112, 16, 18, 53, 162, 127, 158, 130, 152, 133, 138, 12, 170, 159, 129, 127, 4, 141, 115, 134, 158, 132, 41, 98, 90, 76, 15, 88, 101, 162, 165, 124, 128, 31, 75, 86, 90, 161, 108, 100, 162, 102, 47, 150, 42, 78, 138, 154, 40, 99, 49, 175, 69, 165, 46, 1, 178, 165, 86, 129, 115, 178, 142, 144, 53, 163, 36, 66, 161, 157, 153, 62, 24, 15, 123, 147, 38, 146, 104, 44, 5, 171, 160, 20, 155, 19, 164, 165, 43, 53, 77, 129, 137, 116, 132, 59, 90, 19, 142, 137, 37, 97, 95, 11, 85, 39, 162, 134, 76, 91, 56, 129, 172, 135, 176, 74, 109, 49, 55, 63, 155, 131, 155, 33, 120, 140, 134, 132, 94, 122, 36, 134, 178, 162, 65, 133, 57, 133, 80, 177, 67, 132, 112, 63, 25, 122, 103, 145, 164, 14, 87, 136, 80, 46, 150, 55, 45, 154, 79, 56, 60, 143, 6, 145, 124, 157, 84, 116, 46, 137, 130, 132, 161, 165, 28, 24, 44, 148, 41, 141, 50, 44, 40, 36, 21, 6, 10, 36, 65, 145, 41, 148, 42, 179, 42, 26, 156, 164, 34, 62, 48, 32, 2, 8, 40, 98, 164, 139, 91, 17, 61, 28, 106, 21, 76, 159, 116, 88, 30, 137, 28, 73, 132, 135, 124, 53, 1, 111, 7, 151, 9, 156, 14, 178, 135, 5, 40, 34, 108, 5, 33, 65, 41, 64, 128, 145, 51, 37, 138, 48, 21, 67, 167, 129, 149, 161, 31, 28, 41, 1, 58, 9, 23, 36, 91, 43, 145, 122, 142, 159, 4, 148, 172, 40, 27, 162, 92, 137, 29, 79, 70, 62, 17, 144, 177, 48, 78, 8, 122, 140, 130, 104, 162, 1, 111, 129, 95, 124, 152, 151, 142, 148, 151, 167, 171, 27, 15, 11, 53, 13, 40, 32, 19, 15, 179, 8, 177, 172, 128, 142, 132, 11, 139, 6, 174, 172, 27, 180, 172, 146, 40, 174, 4, 93, 45, 60, 49, 40, 167, 43, 154, 59, 48, 41, 28, 50, 16, 56, 25, 49, 84, 55, 50, 178, 121, 128, 81, 80, 15, 22, 177, 16, 114, 165, 34, 158, 70, 13, 169, 17, 138, 11, 19, 1, 115, 144, 145, 34, 161, 131, 33, 31, 153, 28, 4, 28, 96, 79, 33, 127, 127, 146, 103, 112, 143, 170, 50, 83, 148, 35, 82, 94, 144, 97, 71, 156, 159, 127, 132, 40, 158, 7, 144, 140, 26, 118, 83, 41, 49, 67, 52, 60, 61, 41, 36, 169, 133, 14, 87, 80, 95, 68, 99, 29, 61, 112, 113, 11, 90, 57, 41, 86, 72, 13, 47, 53, 7, 28, 59, 179, 60, 34, 148, 52, 47, 172, 150, 147, 100, 119, 136, 125, 86, 111, 74, 106, 93, 139, 140, 176, 100, 114, 178, 25, 161, 43, 61, 24, 34, 10, 28, 48, 38, 5, 15, 14, 163, 144, 138, 26, 153, 142, 15, 34, 142, 26, 154, 27, 147, 3, 44, 171, 27, 146, 18, 39, 55, 63, 146, 174, 147, 143, 141, 145, 156, 149, 139, 77, 53, 46, 42, 43, 28, 56, 164, 114, 77, 132, 86, 115, 130, 90, 120, 143, 36, 7, 180, 37, 8, 85, 58, 97, 95, 142, 133, 11, 32, 145, 105, 177,

158, 164, 179, 168, 94, 65, 76, 71, 141, 79, 76, 93, 24, 83, 23, 107, 119, 131, 130, 155, 171, 102, 172, 42, 24, 85, 64, 63, 50, 63, 69, 38, 168, 158, 77, 72, 91, 130, 81, 41, 126, 36, 62, 123, 92, 21, 89, 169, 25, 174, 35, 134, 86, 37, 55, 101, 122, 109, 98, 78, 90, 169, 60, 38, 152, 84, 179, 64, 72, 101, 114, 154, 29, 38, 44, 76, 117, 124, 139, 113, 38, 123, 103, 85, 131, 120, 90, 84, 88, 113, 61, 88, 106, 101, 150, 163, 79, 5, 150, 166, 16, 53, 164, 62, 165, 0, 176, 7, 24, 31, 161, 62, 161, 61, 77, 72, 93, 20, 96, 90, 74, 124, 19, 19, 99, 42, 38, 30, 170, 46, 49, 54, 80, 74, 97, 47, 52, 117, 9, 67, 108, 135, 138, 153, 17, 150, 43, 175, 91, 1, 84, 119, 32, 71, 31, 21, 28, 48, 161, 166, 88, 99, 146, 133, 120

## 4) Body-axes angles of 1776 cows corresponding to Fig. 2b (angles are measured in degrees from east to west in counter-clockwise sense)

78, 157, 104, 139, 137, 64, 159, 147, 101, 136, 144, 151, 146, 122, 167, 118, 94, 43, 61, 174, 97, 101, 83, 123, 125, 70, 111, 92, 40, 80, 109, 105, 7, 45, 84, 167, 64, 144, 65, 80, 162, 2, 50, 82, 130, 174, 100, 77, 65, 58, 171, 2, 116, 173, 167, 156, 136, 158, 164, 2, 176, 153, 132, 153, 172, 171, 5, 22, 19, 177, 132, 0, 132, 51, 161, 94, 95, 50, 170, 119, 27, 57, 70, 109, 146, 71, 75, 47, 145, 113, 91, 123, 117, 19, 23, 79, 131, 18, 118, 120, 89, 103, 169, 109, 95, 80, 104, 165, 155, 93, 126, 122, 54, 7, 103, 131, 83, 92, 61, 61, 12, 67, 85, 102, 66, 43, 8, 21, 28, 152, 164, 6, 25, 77, 129, 83, 172, 61, 80, 158, 89, 157, 37, 156, 67, 27, 116, 177, 51, 66, 135, 81, 55, 89, 144, 3, 121, 166, 29, 94, 26, 171, 124, 142, 171, 162, 154, 159, 86, 60, 54, 70, 64, 35, 27, 86, 80, 94, 77, 75, 85, 121, 119, 125, 176, 176, 100, 85, 52, 173, 1, 150, 123, 63, 152, 117, 135, 149, 153, 138, 90, 89, 73, 118, 109, 157, 24, 2, 137, 25, 44, 50, 140, 143, 31, 127, 71, 3, 57, 130, 151, 63, 151, 88, 47, 33, 65, 140, 52, 20, 81, 148, 17, 57, 126, 167, 153, 176, 48, 141, 80, 58, 20, 160, 118, 84, 149, 154, 144, 76, 144, 145, 145, 39, 59, 124, 89, 18, 69, 11, 138, 101, 68, 14, 40, 58, 39, 140, 105, 60, 54, 105, 64, 65, 39, 84, 58, 76, 177, 63, 46, 19, 57, 50, 177, 36, 36, 63, 176, 164, 20, 12, 73, 165, 16, 77, 23, 130, 55, 45, 42, 65, 33, 36, 54, 113, 111, 85, 10, 110, 127, 84, 132, 173, 24, 61, 40, 36, 138, 165, 28, 139, 34, 37, 47, 100, 145, 46, 34, 63, 75, 47, 145, 116, 141, 51, 124, 53, 93, 141, 106, 5, 11, 32, 23, 133, 117, 91, 72, 91, 30, 35, 91, 157, 168, 60, 51, 87, 37, 10, 141, 64, 98, 143, 67, 173, 93, 120, 139, 100, 119, 125, 12, 113, 93, 140, 143, 44, 50, 138, 132, 137, 138, 84, 145, 127, 20, 134, 85, 91, 42, 179, 52, 53, 30, 175, 50, 152, 91, 138, 146, 124, 143, 141, 178, 173, 46, 125, 160, 91, 146, 158, 145, 113, 53, 43, 83, 104, 53, 147, 92, 171, 152, 152, 118, 57, 47, 44, 3, 47, 165, 41, 164, 152, 156, 113, 1, 158, 38, 158, 108, 144, 94, 43, 39, 41, 96, 38, 9, 68, 42, 38, 34, 30, 31, 34, 0, 99, 47, 0, 95, 127, 149, 135, 44, 121, 48, 98, 88, 124, 12, 39, 46, 71, 65, 43, 97, 39, 161, 145, 164, 172, 47, 125, 102, 35, 72, 54, 143, 115, 128, 50, 62, 126, 136, 38, 42, 51, 139, 170, 76, 35, 144, 148, 35, 39, 116, 64, 121, 67, 30, 121, 116, 62, 30, 175, 122, 45, 138, 140, 160, 93, 121, 132, 31, 43, 139, 87, 119, 56, 86, 99, 45, 68, 133, 108, 72, 122, 171, 72, 63, 120, 109, 25, 129, 137, 41, 126, 40, 88, 79, 71, 74, 71, 101, 75, 79, 24, 154, 43, 163, 68, 110, 150, 39, 125, 54, 153, 155, 75, 84, 59, 20, 177, 43, 59, 50, 24, 123, 129, 127, 70, 86, 86, 60, 108, 139, 155, 51, 97, 66, 43, 98, 99, 150, 40, 135, 128, 174, 40, 17, 61, 88, 149, 39, 104, 49, 81, 0, 53, 37, 144, 114, 99, 87, 86, 57, 83, 74, 49, 28, 147, 59, 111, 104, 150, 104, 29, 63, 45, 86, 65, 81, 70, 69, 104, 105, 52, 124, 63, 82, 53, 43, 128, 86, 62, 51, 47, 54, 46, 82, 79, 173, 47, 48, 39, 65, 89, 68, 30, 115, 63, 28, 69, 171, 97, 22, 36, 47, 110, 88, 61, 41, 179, 43, 16, 37, 87, 51, 64, 161, 105, 87, 9, 8, 63, 27, 166, 103, 132, 131, 141, 92, 117, 120, 48, 123, 142, 127, 140, 26, 98, 141, 49, 43, 136, 153, 40, 42, 35, 17, 46, 146, 15, 143, 55, 51, 31, 31, 57, 75, 46, 53, 43, 178, 77, 62, 68, 72, 74, 76, 67, 84, 96, 125, 128, 131, 116, 12, 131, 104, 75, 61, 71, 170, 66, 96, 37, 163, 25, 17, 65, 53, 63, 41, 7, 104, 137, 156, 119, 165, 125, 117, 155, 170, 96, 76, 98, 98, 135, 58, 133, 69, 98, 99, 103, 107, 45, 117, 72, 68, 44, 86, 70, 143, 117, 63, 91, 66, 60, 89, 62, 54, 92, 176, 87, 63, 79, 114, 148, 59, 42, 58, 97, 106, 54, 153, 53, 124, 15, 74, 100, 60, 80, 123, 125, 77, 67, 54, 165, 159, 149, 169, 77, 132, 127, 157, 168, 107, 135, 123, 127, 123, 136, 154, 164, 175, 0, 137, 137, 117, 75, 94, 96, 126, 89, 90, 108, 30, 81, 53, 36, 28, 128, 105, 54, 70, 85, 31, 139, 139, 92, 145, 80, 135, 38, 118, 40, 85, 107, 21, 46, 112, 135, 52, 140, 124, 133, 75, 69, 142, 156, 144, 117, 77, 157, 133, 41, 18, 40, 40, 10, 54, 76, 138, 119, 33, 41, 39, 176, 24, 32, 113, 68, 8, 21, 169, 13, 79, 6, 62, 89, 37, 113, 113, 116, 43, 125, 32, 61, 80, 103, 27, 84, 2, 36, 58, 49, 23, 6, 9, 90, 170, 141, 65, 47, 91, 174, 58, 60, 52, 68, 65, 48, 38, 41, 46, 40, 65, 178, 131, 57, 90, 43, 60, 54, 107, 161, 55, 145, 137, 72, 72, 121, 131, 151, 19, 129, 26, 40, 127, 83, 75, 9, 10, 114, 160, 9, 30, 136, 78, 164, 11, 153, 7, 167, 159, 5, 175, 174, 147, 180, 100, 100, 19, 5, 131, 45, 86, 162, 141, 60, 100, 145, 64, 120, 2, 38, 81, 45, 66, 48, 77, 1, 14, 7, 65, 68, 151, 167, 141, 151, 145, 132, 90, 143, 152, 168, 156, 12, 138, 102, 49, 165, 168, 154, 29, 37, 176, 160, 104, 5, 31, 76, 55, 77, 82, 6, 158, 1, 79, 38, 89, 68, 128, 47, 54, 45, 63, 92, 170, 175, 146, 37, 145, 72, 169, 14, 102, 108, 180, 175, 0, 143, 120, 170, 169, 167, 20, 158, 54, 161, 55, 148, 40, 123, 165, 30, 172, 122, 120, 99, 90, 40, 60, 160, 0, 26, 31, 25, 14, 14, 173, 27, 141, 28, 62, 160, 154, 134, 129, 149, 114, 143, 130, 156, 141, 147, 165, 157, 170, 105, 135, 115, 147, 93, 146, 125, 156, 168, 87, 146, 152, 5, 10, 19, 32, 37, 6, 63, 52, 116, 14, 72, 20, 61, 39, 119, 140, 98, 83, 85, 138, 19, 68, 36, 133, 16, 14, 8, 162, 95, 1, 140, 135, 37, 134, 129, 171, 21, 106, 0, 129, 143, 149, 77, 40, 175, 117, 34, 18, 160, 58, 108, 28, 89, 175, 76, 103, 159, 120, 77, 25, 32, 24, 56, 58, 75, 103, 51, 14, 136, 150, 170, 92, 24, 179, 155, 147, 154, 156, 162, 4, 168, 162, 167, 175, 19, 92, 70, 76, 71, 100, 129, 92, 67, 92, 101, 176, 29, 163, 161, 128, 165, 172, 120, 121, 45, 11, 59, 88, 173, 120, 41, 6, 175, 55, 159, 52, 31, 34, 93, 35, 90, 140, 154, 40, 72, 89, 56, 143, 159, 30, 49, 43, 86, 154, 168, 176, 96, 67, 87, 25, 19, 148, 176, 171, 89, 40, 37, 7, 82, 76, 93, 47, 44, 45, 53, 42, 179, 24, 10, 3, 107, 64, 3, 161, 168, 58, 57, 38, 49, 73, 112, 173, 87, 32, 51, 114, 0, 149, 121, 118, 137, 86, 168, 66, 98, 56, 161, 68, 69, 172, 41, 78, 94, 95, 107, 97, 137, 124, 50, 101, 107, 80, 76, 175, 152, 62, 4, 117, 125, 168, 127, 68, 54, 94, 174, 175, 76, 164, 129, 116, 124, 117, 151, 72, 168, 150, 140, 127, 70, 103, 6, 0, 58, 96, 143, 48, 38, 50, 124, 48, 76, 103, 13, 50, 144, 57, 34, 35, 54, 171, 149, 51, 48, 94, 78, 46, 126, 37, 84, 63, 67, 5, 42, 64, 62, 83, 93, 43, 75, 87, 49, 36, 109, 55, 36, 72, 103, 96, 14, 140, 140, 57, 145, 88, 122, 103, 86, 68, 89, 137, 22, 31, 14, 55, 134, 35, 24, 50, 139, 166, 94, 39, 9, 39, 130, 54, 36, 47, 0, 119, 18, 163, 38, 168, 136, 28, 0, 0, 144, 98, 153, 130, 145, 151, 9, 0, 157, 171, 144, 106, 175, 166, 169, 37, 141, 106, 25, 86, 84, 110, 51, 91, 55, 33, 16, 92, 101, 58, 52, 58, 150, 160, 152, 32, 136, 42, 65, 85, 28, 35, 156, 29, 139, 2, 104, 105, 42, 51, 74, 121, 95, 151, 86, 74, 147, 105, 55, 135, 106, 122, 99, 32, 134, 143, 112, 17, 78, 60, 46, 160, 3, 0, 8, 83, 119, 55, 22, 142, 72, 125, 77, 125, 0, 56, 111, 131, 60, 55, 153, 126, 147, 40, 39, 103, 166, 32, 12, 62, 108, 35, 154, 28, 172, 151, 132, 121, 119, 157, 162, 132, 14, 102, 155, 132, 146, 140, 78, 62, 91, 137, 39, 20, 96, 111, 57, 90, 128, 127, 62, 47, 48, 79, 104, 138, 77, 129, 33, 54, 12, 93, 71, 39, 105, 149, 154, 36, 55, 30, 102, 53, 90, 123, 61, 154, 139, 142, 126, 145, 131, 65, 123, 126, 99, 94, 128, 139, 95, 137, 123, 126, 130, 131, 147, 142, 120, 157, 124, 121, 149, 105, 133, 141, 106, 128, 161, 123, 156, 165, 127, 138, 153, 140, 121, 145, 123, 124, 91, 106, 0, 133, 171, 138, 89, 44, 71, 25, 91, 54, 170, 77, 128, 90, 114, 121, 17, 0, 152, 152, 119, 121, 85, 95, 135, 69, 0, 172, 134, 83, 78, 52, 38, 79, 63, 36, 81, 107, 25, 134, 59, 72, 160, 28, 0, 141, 13, 20, 117, 5, 53, 138, 15, 169, 0, 24, 141, 123, 45, 127, 143, 0, 11, 106, 39, 111, 73, 124, 0, 100, 130, 46, 113, 107, 102, 115, 87, 104, 46, 117, 68, 37, 46, 151, 172, 154, 173, 130, 136, 141, 44, 31, 159, 157, 130, 45, 121, 108, 81, 72, 133, 138, 141, 124, 99, 0, 145, 89, 89, 73, 59, 136, 76, 136, 76, 170, 126, 5, 150, 90, 102, 31, 17, 88, 93, 28, 108, 138, 82, 129, 106, 144, 83, 51, 141, 113, 85, 87, 6, 0, 115, 141, 108, 99, 120, 56, 95, 124, 109, 146

## 5) Body-vector angles of 589 cows corresponding to Fig. 4 (angles are measured in degrees from east to west in counter-clockwise sense)

237, 86, 249, 253, 274, 244, 270, 111, 125, 287, 277, 249, 294, 107, 275, 95, 73, 112, 285, 269, 308, 254, 267, 310, 123, 184, 311, 176, 124, 148, 124, 61, 303, 72, 233, 243, 249, 56, 249, 251, 280, 255, 53, 319, 230, 223, 271, 85, 248, 237, 73, 342, 333, 262, 338, 112, 126, 226, 153, 13, 87, 288, 278, 282, 199, 124, 108, 108, 200, 122, 123, 55, 206, 329, 51, 189, 210, 32, 48, 161, 26, 63, 333, 183, 165, 256, 157, 289, 291, 319, 313, 309, 295, 267, 267, 263, 159, 210, 92, 82, 92, 42, 87, 228, 288, 98, 243, 220, 206, 205, 260, 144, 247, 334, 242, 306, 297,

242, 339, 10, 262, 58, 254, 354, 273, 169, 313, 352, 351, 20, 330, 157, 285, 272, 241, 4, 332, 180, 263, 120, 99, 184, 254, 232, 32, 56, 224, 198, 190, 140, 138, 344, 237, 297, 201, 302, 281, 109, 169, 63, 266, 326, 226, 339, 356, 216, 320, 351, 164, 196, 83, 285, 84, 31, 258, 266, 259, 255, 263, 78, 276, 133, 320, 307, 275, 167, 264, 204, 193, 28, 142, 84, 217, 244, 170, 337, 137, 61, 153, 83, 74, 176, 143, 160, 169, 108, 174, 125, 139, 162, 161, 152, 324, 213, 285, 202, 173, 334, 255, 55, 310, 57, 37, 111, 42, 131, 132, 338, 308, 8, 32, 337, 351, 142, 132, 147, 91, 175, 143, 158, 174, 244, 123, 154, 126, 138, 167, 175, 203, 183, 185, 175, 168, 168, 182, 206, 182, 185, 124, 89, 95, 131, 170, 112, 158, 102, 137, 206, 189, 131, 169, 197, 180, 356, 25, 282, 350, 256, 127, 258, 321, 237, 180, 359, 297, 239, 246, 245, 261, 247, 200, 294, 300, 102, 136, 102, 65, 107, 116, 67, 237, 49, 73, 307, 66, 42, 122, 19, 279, 211, 30, 27, 53, 339, 114, 96, 95, 116, 45, 39, 259, 257, 47, 272, 69, 219, 280, 43, 89, 136, 123, 184, 210, 113, 106, 118, 310, 276, 43, 138, 138, 41, 35, 33, 163, 349, 276, 286, 303, 297, 268, 249, 331, 208, 234, 268, 249, 176, 338, 6, 17, 57, 167, 132, 345, 124, 23, 340, 340, 46, 56, 79, 128, 132, 109, 132, 60, 94, 197, 147, 142, 135, 83, 229, 329, 52, 228, 153, 258, 235, 62, 140, 182, 325, 302, 151, 83, 292, 49, 139, 133, 134, 158, 167, 209, 207, 224, 327, 222, 139, 235, 46, 23, 165, 275, 136, 27, 78, 71, 58, 201, 320, 353, 47, 74, 186, 121, 145, 133, 103, 161, 181, 105, 125, 95, 128, 151, 150, 142, 147, 149, 170, 177, 200, 197, 189, 234, 195, 221, 214, 198, 194, 182, 195, 173, 167, 130, 143, 130, 194, 134, 182, 172, 173, 206, 178, 172, 151, 218, 176, 185, 96, 48, 233, 51, 41, 164, 37, 148, 65, 54, 224, 30, 45, 193, 58, 24, 231, 85, 54, 235, 178, 120, 126, 83, 84, 193, 208, 357, 20, 109, 161, 37, 159, 69, 193, 354, 23, 319, 196, 199, 183, 115, 139, 146, 210, 159, 135, 36, 36, 153, 23, 187, 31, 100, 77, 36, 127, 127, 143, 280, 297, 323, 350, 50, 79, 153, 211, 258, 269, 318, 278, 254, 158, 156, 308, 312, 36, 159, 8, 327, 320, 25, 292, 84, 108, 101, 152, 167, 260, 190, 152, 342, 20, 58, 166, 243, 343, 181, 1, 5, 23, 32, 342, 60, 166, 238, 252, 251, 276, 203, 277, 266, 257, 129, 200, 200, 98, 43

## 6) Figure showing one of the measured herds. The 25 shown cows correspond to 25 first body-axes angles from point (4)

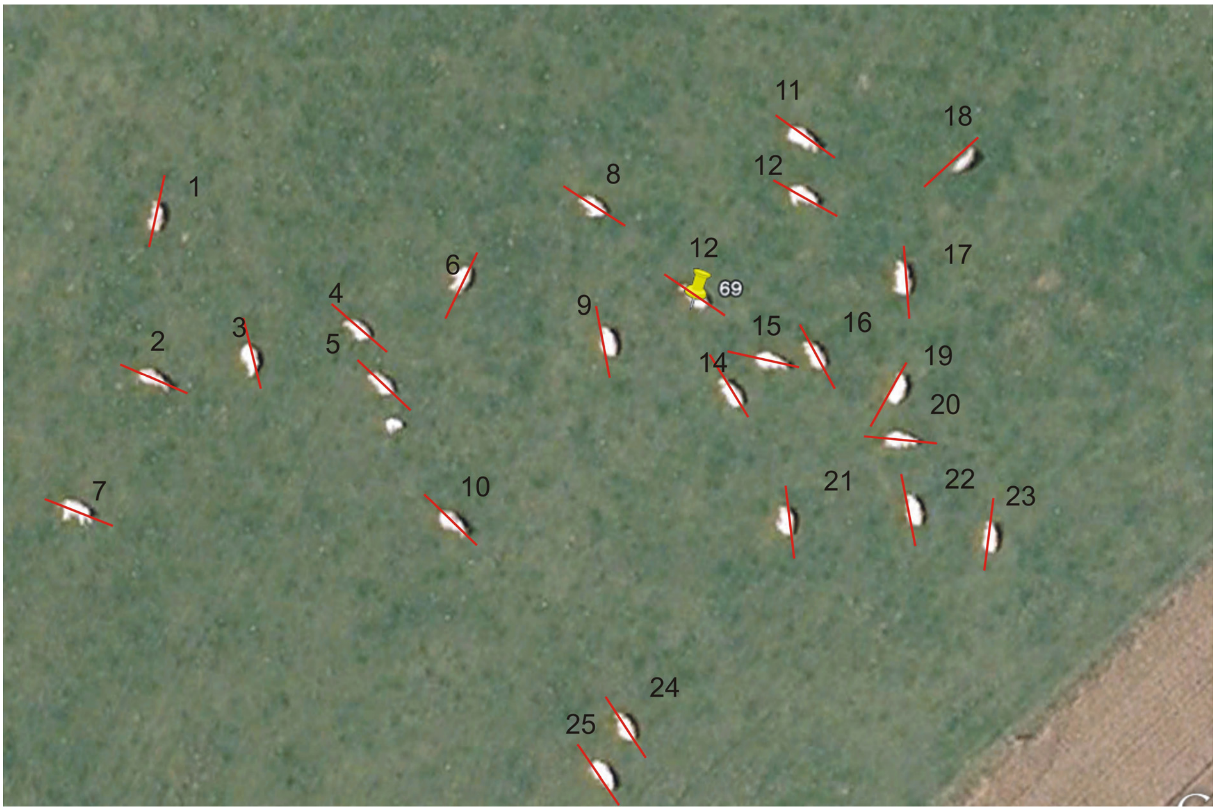


## 7) Coordinates of measured herds in WGS 84 system

(N54º57'8"E-1º46'26"), (N54º59'34"E-1º38'6"), (N54º35'3"E-1º50'50"), (N54º34'37"E-1º50'54"), (N54º32'15"E-1º49'10"), (N54º29'3"E-1º48'28"), (N53º54'50"E-1º36'1"), (N53º50'57"E-1º29'55"), (N53º51'50"E-1º56'5"), (N53º51'24"E-1º56'58"), (N53º49'8"E-2º34'31"), (N53º42'53"E-2º35'53"), (N53º42'26"E-2º37'3"), (N53º42'24"E-2º37'8"), (N53º41'54"E-2º37'30"), (N53º24'19"E-1º33'7"), (N53º20'57"E-1º40'33"), (N53º10'50"E-2º47'57"), (N53º10'37"E-2º47'53"), (N53º10'26"E-2º48'3"), (N53º7'59"E-2º50'26"), (N53º8'31"E-2º46'26"), (N53º8'39"E-2º45'55"), (N53º1'6"E0º56'59"), (N53º1'8"E0º56'56"), (N52º26'7"E-2º43'53"), (N52º12'36"E-2º31'57"), (N52º5'21"E-2º28'59"), (N51º59'23"E-2º59'31"), (N51º52'28"E-2º52'53"), (N51º50'55"E-2º48'16"), (N52º16'9"E-1º18'15"), (N52º16'2"E-1º17'46"), (N52º15'48"E-1º18'5"), (N51º47'55"E0º17'38"), (N51º32'25"E0º29'38"), (N51º30'22"E0º25'29"), (N50º43'38"E-2º25'42"), (N50º43'36"E-2º26'11"), (N50º44'41"E-2º27'59"), (N50º44'46"E-2º28'8"), (N50º54'41"E-3º40'18"), (N50º59'12"E-3º43'2"), (N56º17'43"E-2º49'9"), (N56º18'14"E-2º48'56"), (N56º19'21"E-2º48'38"), (N56º20'37"E-2º49'9"), (N57º2'1"E-2º35'11"), (N57º0'45"E-2º12'38"), (N57º1'8"E-2º10'27"), (N54º22'43"E-4º27'21"), (N54º21'21"E-4º27'11"), (N54º19'32"E-4º27'51"), (N54º13'11"E-4º40'50"), (N54º10'28"E-4º32'19"), (N54º7'28"E-4º38'18"), (N54º6'33"E-4º36'40"), (N54º6'38"E-4º40'37"), (N54º5'38"E-4º43'55"), (N54º5'50"E-4º45'25"), (N48º11'53"E-1º36'9"), (N48º11'36"E-1º37'50"), (N48º11'13"E-1º39'13"), (N48º9'26"E-1º36'25"), (N48º8'45"E-1º36'31"), (N48º8'0"E-1º36'2"), (N48º6'32"E-1º35'11"), (N49º8'28"E0º14'7"), (N49º15'28"E0º19'50"), (N49º16'43"E0º21'6"), (N49º15'38"E0º14'31"), (N49º14'57"E0º15'50"), (N49º14'42"E0º15'34"), (N49º22'32"E0º20'56"), (N49º22'50"E0º20'20"), (N51º35'34"E5º26'59"), (N52º6'52"E5º10'0"), (N52º7'24"E5º9'51"), (N52º23'18"E6º20'36"), (N47º1'39"E7º18'13"), (N47º1'29"E7º22'10"), (N47º0'9"E7º23'51"), (N47º1'11"E7º25'29"), (N46º59'31"E7º26'33"), (N50º29'2"E13º21'15"), (N50º13'27"E12º23'11"), (N50º12'52"E12º25'54"), (N49º4'28"E14º0'51"), (N48º58'49"E13º54'36"), (N48º56'52"E13º58'39"), (N48º53'35"E13º54'33"), (N48º45'6"E13º58'7"), (N48º43'59"E14º0'23"), (N48º42'37"E14º0'52"), (N48º39'4"E14º26'29"), (N48º39'23"E14º35'0"), (N48º46'58"E14º42'26"), (N48º47'9"E14º47'53"), (N49º8'8"E17º58'40"),

(N49º45'57"E17º38'12"), (N49º46'3"E17º38'16"), (N48º47'10"E14º48'22"), (N48º48'5"E0º28'57"), (N48º6'36"E-1º34'23"), (N48º1'46"E-1º37'43"), (N48º9'50"E-1º47'16"), (N48º11'23"E-1º45'7"), (N48º11'47"E-1º44'24"), (N48º4'54"E-1º32'22"), (N48º11'21"E-1º45'14"), (N49º32'47"E0º08'33"), (N49º31'20"E0º17'02"), (N49º61'22"E0º18'14"), (N49º33'33"E0º20'08"), (N49º34'12"E0º19'53"), (N49º31'44"E0º17'08"), (N49º31'23"E0º18'14"), (N49º33'33"E0º15'29"), (N49º30'34"E0º20'51"), (N49º25'07"E0º24'58"), (N50º43'33"E2º25'59"), (N53º43'34"E2º26'01"), (N50º43'38"E2º25'42"), (N50º44'42"E2º27'59"), (N50º46'25"E2º16'11"), (N50º12'53"E12º25'55"), (N50º28'54"E13º21'00"), (N50º29'02"E13º21'15"), (N50º13'25"E12º23'09"), (N50º43'55"E2º29'02"), (N49º31'58"E0º16'14"), (N19º22'14"E0º10'21"), (N49º24'48"E0º17'55"), (N49º24'13"E0º12'09"), (N49º34'05"E0º14'44"), (N49º31'55"E0º15'58"), (N49º29'56"E0º21'43"), (N49º29'22"E0º22'04"), (N49º24'51"E0º24'29"), (N49º30'21"E0º23'31"), (N49º25'05"E0º22'50"), (N49º25'04"E0º19'47"), (N49º25'04"E0º19'47"), (N51º44'27"E5º11'06"), (N51º44'42"E5º09'12"), (N51º44'39"E5º09'20"), (N51º44'22"E5º09'06"), (N51º45'59"E5º07'55"), (N51º44'24"E5º07'04"), (N50º06'08"E5º35'47"), (N50º04'22"E5º41'43"), (N50º04'10"E5º40'43"), (N50º03'58"E5º40'41"), (N50º04'10"E5º40'41"), (N50º03'14"E5º39'13"), (N51º44'35"E5º05'34"), (N51º44'56"E5º04'17"), (N51º44'44"E5º04'02"), (N51º50'33"E5º02'04"), (N51º49'27"E5º00'39"), (N51º51'57"E4º58'46"), (N51º53'50"E4º58'42"), (N51º54'19"E4º57'22"), (N50º04'14"E5º39'55"), (N50º05'07"E5º41'06"), (N50º05'33"E5º39'51"), (N50º04'54"E5º39'37"), (N50º04'31"E5º39'16"), (N51º44'27"E5º11'06"), (N53º04'24"E5º46'59"), (N53º04'22"E5º47'19"), (N53º04'50"E5º47'07"), (N53º05'36"E5º44'52"), (N53º06'29"E5º44'47"), (N53º00'57"E5º46'73"), (N52º59'31"E5º49'32"), (N52º59'31"E5º51'04"), (N52º59'31"E5º51'04"), (N52º19'06"E6º00'50"), (N52º20'05"E6º03'19"), (N52º20'56"E6º05'13"), (N51º58'23"E5º07'24"), (N51º02'42"E5º02'42"), (N48º43'09"E14º23'07"), (N48º43'18"E14º16'36"), (N49º07'44"E13º44'50"), (N49º10'29"E13º44'35"), (N43º11'76"E13º44'21"), (N48º56'46"E13º58'26"), (N48º54'53"E14º01'04"), (N48º56'04"E14º09'38"), (N56º22'33"E8º41'55"), (N53º36'34"E12º27'27"), (N53º36'34"E12º23'21"), (N53º35'01"E13º15'12"), (N53º36'07"E13º26'41"), (N52º52'46"E12º31'17"), (N52º29'52"E8º30'32"), (N52º30'25"E8º31'55"), (N52º30'33"E8º31'43"), (N52º30'54"E8º32'43"), (N52º31'11"E8º31'28"), (N52º24'28"E8º12'07"), (N53º43'53"E9º51'14"), (N53º45'00"E9º54'51"), (N47º05'32"E7º44'08"), (N47º05'17"E7º45'14"), (N47º05'29"E7º46'09"), (N47º31'40"E7º49'58"), (N47º05'00"E7º49'14"), (N47º05'11"E7º49'26"), (N47º08'41"E7º53'08"), (N47º09'23"E7º37'54"), (N47º01'49"E7º40'46"),
